# Supplementary material for: Unimodal Mono-Partite Matching in a Bandit Setting
Source: arXiv:2208.01511 source file (2022-08-02)
Supplement: Supplementary file 1 [file supplementary_content.tex]

The appendix is organized as follows. We first list most of the notations used in the paper in Appendix \ref{app:notations}. Lemma \ref{lem:pbm_is_unimodal} is proved in Appendix \ref{app:pbm_is_unimodal}. In Appendix \ref{app:prelim}, we recall a Lemma from \cite{Combes2014} used by our own Lemmas and Theorems, and then in Appendices \ref{app:good_leader} to \ref{app:badordering} we respectively prove Theorem \ref{theo:good_leader}, Lemma \ref{lem:bad_leader}, and Lemma \ref{lem:badordering}. In Appendix \ref{app:KL-Comb_to_PBM} we define KL-CombUCB and discuss its regret and its relation to \ouralgo{}. Finally in Appendix \ref{app:fgrab} we introduce and discuss \ouralgofull{}.

\section{Notations}\label{app:notations}

The following table summarize the notations used through the paper and the appendix.

%\begin{center}
%    \begin{small}
%        \begin{sc}
%            \begin{longtable}{ll}
%                \toprule
%                \textbf{Symbol} & \textbf{Meaning}                 \\
%                \midrule
%                \endhead
%
%                \hline \multicolumn{2}{r}{{Continued on next page}}
%                \endfoot
%
%                \bottomrule
%                \endlastfoot
%
%                \horizon        & Time horizon                     \\
%                \iteration      & Iteration                        \\
%                \nitems         & Number of items                  \\
%                \index          & index of an item                 \\
%                \intset{n}      & Set of integer $\{1,\dots , n\}$ \\
%                \carm{t}        & $\dots$                          \\
%                \leader{t}      & $\dots$                          \\
%                \optimum        & $\dots$                          \\
%            \end{longtable}
%        \end{sc}
%    \end{small}
%\end{center}

\begin{center}
\begin{small}
\begin{sc}
    \begin{longtable}{ll}
        \toprule
        \textbf{Symbol} &\textbf{Meaning}\\
        \midrule
        \endhead
        
        \hline \multicolumn{2}{r}{{Continued on next page}}
        \endfoot
        
        \bottomrule
        \endlastfoot

         T& Time horizon\\
        $t$& iteration \\
        L& number of items \\
        $i$& index of an item \\
        K& number of positions in a recommendation\\
        $k$ & index of a position \\
        $[n]$ & set of integers $\{1,\dots,n\}$\\
        $\perm_K^L$ & set of permutations of K distinct items among L\\
        $\thetav$& vectors of probabilities of click\\
        $\theta_i$& probability of click on item $i$ \\
        $\kappav$& vectors of probabilities of view \\
        $\kappa_k$& probability of view at position $k$ \\
        $\Ac$ & set of bandit arms\\
        $\av$ & an arm in  $\Ac$ \\
        $\av(t)$ & the arm chosen at iteration $t$ \\
        $\tilde \av(t)$ & best arm at iteration $t$ given the previous choices and feedbacks (called leader)  \\
        $\av^*$ & best arm \\
        $G$ & graph carrying a partial order on $\Ac$ \\
        $\gamma$ & maximum degree of $G$ \\
        $\Nc_G(\tilde \av(t))$ & neighborhood of $\tilde a(t)$ given $G$ \\
        $\rho_{i,k}$& probability of click on item $i$ displayed at position $k$ \\
        $\cv(t)$& clicks vector at iteration $t$ \\
        $r(t)$ & reward collected at iteration $t$, $r(t)=\sum_{k=1}^K c_k(t)$\\
        $\mu_\av$& expectation of $r(t)$ while recommending $\av$, $\mu_\av=\sum_{k=1}^K \rho_{a_k,k}$ \\
        $\mu^*$& highest expected reward, $\mu^*=\max_{\av\in \perm_K^L}\mu_\av$\\
        $\Delta_a$& gap between $\mu_a$ and $\mu^*$ \\
        $\Delta_{min}$& minimal value for $\Delta_a$\\ 
        $\Delta$& generic reward gap between one of the sub-optimal arms and one of the best arms\\
        $R(T)$ & cumulative (pseudo-)regret, $R(T) = T\mu^* - \EE\left[\sum_{t = 1}^T \mu_{\av(t)}\right]$\\
        $\Pi_\rhov(\av)$& set of permutations in $\perm_K^K$ ordering the positions s.t. $\rho_{a_{\pi_{1}},\pi_{1}} \geqslant \rho_{a_{\pi_{2}},\pi_{2}} \geqslant \dots \geqslant \rho_{a_{\pi_{K}},\pi_{K}}$\\
        $\piv$& element of  $\Pi_\rhov(\av)$\\
        $\tilde\piv$& estimation of $\piv$\\
        $\av \circ (\pi_{k}, \pi_{k+1})$ & permutation swapping items in positions $\pi_{k}$ and $\pi_{k+1}$\\
        $\av[\pi_{K} := i]$& permutation leaving $\av$ the same for any position except $\pi_{K}$ for which $\av[\pi_{K}~:=~i]_{\pi_{K}}=i$\\
        ${\mapping}$ & rankings of positions respecting $\Pi_\rhov$,  ${\mapping} =\left(\piv_\av\right)_{\av \in \perm_K^L}$ s.t. $\forall \av\in \perm_K^L, \piv_\av\in\Pi_\rhov(\av)$\\
        $T_{i,k}(t)$ & number of iterations s.t. item $i$ has been displayed at position $k$, $T_{i,k}(t) = \sum_{s = 1}^{t-1} \ind\{a_k(s) = i\}$\\
        $\tilde{T}_\av(t)$ &  number of iterations s.t. the leader was $\av$, $\tilde{T}_\av(t) \defeq \sum_{s = 1}^{t-1} \ind\{\tilde\av(s) = \av\}$ \\
        $T_\av(t)$ &  number of iterations s.t. the chosen arm was $\av$, $T_\av(t) = \sum_{s = 1}^{t-1} \ind\{\av(s) = \av\}$ \\
        $T_\av^{\tilde\av}(t)$ & number of iterations s.t. the leader was $\tilde\av$, the chosen arm was $\av$, and $\av$ was chosen
        \\& by the argmax on $\sum_{k=1}^K b_{a_k, k}(t)$: $T_{\av}^{\tilde\av}(t) = \sum_{s=1}^{t-1} \ind\left\{\tilde\av(s)=\tilde\av, \av(s) = \av, \tilde{T}_{\tilde\av}(s)/L \notin \NN\right\}$\\
        $\hat\rho_{i,k}(t)$& estimation of $\rho_{i,k}$ at iteration $t$,  $\hat\rho_{i,k}(t) = \frac{1}{T_{i,k}(t)}\sum_{s = 1}^{t-1} \ind\{a_k(s) = i\}c_k(s)$\\
        $b_{i,k}(t)$ & Kullback-Leibler index of $\hat\rho_{i,k}(t)$ , $b_{i,k}(t) = f\left(\hat\rho_{i,k}(t), T_{i,k}(t), \tilde{T}_{\tilde\av(t)}(t)+1\right)$ \\
        $f$ & Kullback-Leibler index function, $f(\hat\rho, s, t) = \sup \{p\in[\hat\rho,1]: s\times\KL(\hat{\rho}, p) \leq \log (t) + 3 \log(\log (t))\},$\\
        $\KL(p,q)$ & Kullback-Leibler divergence from a Bernoulli distribution of mean $p$\\
        &to a Bernoulli distribution of mean $q$,  $\KL(p,q) = p \log \left(\frac{p}{q}\right) + (1-p)\log \left(\frac{1 - p}{1 - q}\right)$ \\
        $B_{\av}(t)$ & pseudo-sum of indices of $\av$ at iteration t, $B_{\av}(t) = \sum_{k=1}^K b_{a_k, k}(t) - \sum_{k=1}^K b_{\tilde{a}_k(t), k}(t)$\\
        $\Nc_{\pi^*}(a^*)$& neighborhood of the best arm\\
%        $P^L_K$& number of K-permutations of L items\\
%        $P_{max}$& size of the larger set of $\Pi_\rhov(\av)$\\
        $K_\av$& (with combinatorial bandit setting) number of elements in $\av$ but not in $\av^*$,\\& $K_\av = \min_{\av^*\in\Ac: \mu_{\av^*}=\mu^*} |\av\setminus\av^*|$\\
        $K_{max}$& (with combinatorial bandit setting) maximal number of elements in a sub-optimal arm $\av$\\& but not in an optimal arm $a^*$, $K_{max}=\max_{\av \in\Ac: \mu_\av\neq\mu^*} K_\av$\\
        $c^*\left(\thetav, \kappav\right)$ & coefficient in the regret bound of PMED\\
        $c$ & (in $\varepsilon_n$-greedy) parameter controlling the probability of exploration\\
        $c$ & (in PB-MHB) parameter controlling size of the step in the Metropolis Hasting inference \\
        $m$ & (in PB-MHB) number of step in the Metropolis Hasting inference \\
\end{longtable}
\end{sc}
\end{small}
\end{center}

\section{Proof of Lemma \ref{lem:pbm_is_unimodal} (PBM Fulfills Assumption 1) }\label{app:pbm_is_unimodal}

\begin{proof}[Proof of Lemma \ref{lem:pbm_is_unimodal}]
Let $(L, K, (\rho_{i,k})_{(i,k)\in [L]\times[K]})$ be an online learning to rank (OLR) problem with users following PBM, with positive probabilities of looking at a given position. Therefore, there exists $\thetav\in[0,1]^L$ and $\kappav\in(0,1]^K$ such that for any item $i$ and any position $k$, $\rho_{i,k}=\theta_i\kappa_k$.

Let $\av\in\perm_K^L$ be a recommendation, and let $\piv\in \Pi_\rhov\left(\av\right)$ be an appropriate ranking of positions. One of the four following properties is satisfied:
\begin{align}
    &\exists k \in [K-1]\text{ s.t. } \theta_{a_{\pi_k}} < \theta_{a_{\pi_{k+1}}}, \label{eq:thetabadinside}\\
    &\exists k \in [K-1]\text{ s.t. } \kappa_{\pi_k} < \kappa_{\pi_{k+1}},\label{eq:kappabad}\\
    &\exists i \in [L]\setminus\av([K])\text{ s.t. } \theta_{a_{\pi_K}} < \theta_{i},\label{eq:thetabadoutside}\\
    &\begin{cases}
        \forall k \in [K-1], \theta_{a_{\pi_k}} \geqslant  \theta_{a_{\pi_{k+1}}}\\
        \forall k \in [K-1], \kappa_{\pi_k} \geqslant \kappa_{\pi_{k+1}}\\
        \forall i \in [L]\setminus\av([K]), \theta_{a_{\pi_K}} \geqslant \theta_{i}
    \end{cases}\label{eq:everythingok}.
\end{align}

Let prove, by considering each of these properties one by one, that $\av$ is either one of the best arms, or $\av$ fulfills either Property (2) or Property (3) of Assumption 1.

If Property \eqref{eq:thetabadinside} is satisfied and $\theta_{a_{\pi_k}}=0$, then by definition of $\piv$ and $\Pi_\rhov\left(\av\right)$, $0=\theta_{a_{\pi_k}}\kappa_{\pi_k} \geqslant \theta_{a_{\pi_{k+1}}}\kappa_{\pi_{k+1}} >0$ which is absurd. 

Therefore, If Property \eqref{eq:thetabadinside} is satisfied, $\frac{\theta_{a_{\pi_{k+1}}}}{\theta_{a_{\pi_k}}} > 1.$

Note that by definition of $\piv$ and $\Pi_\rhov\left(\av\right)$, and as $\rho_{i,k}=\theta_i\kappa_k$,
$\theta_{a_{\pi_k}}\kappa_{\pi_k} \geqslant \theta_{a_{\pi_{k+1}}}\kappa_{\pi_{k+1}}$.

Hence $\kappa_{\pi_k} \geqslant \frac{\theta_{a_{\pi_{k+1}}}}{\theta_{a_{\pi_k}}} \kappa_{\pi_{k+1}} > \kappa_{\pi_{k+1}}$,
and
\begin{align*}
    \mu_\av - \mu_{\av\circ\left(\pi_k, \pi_{k+1}\right)}
    &=  \theta_{a_{\pi_k}}\kappa_{\pi_k} + \theta_{a_{\pi_{k+1}}}\kappa_{\pi_{k+1}}
    - \left(\theta_{a_{\pi_{k+1}}}\kappa_{\pi_k} + \theta_{a_{\pi_k}}\kappa_{\pi_{k+1}}\right)
    \\
    &= \left(\theta_{a_{\pi_k}} - \theta_{a_{\pi_{k+1}}}\right)
    \left(\kappa_{\pi_k} - \kappa_{\pi_{k+1}}\right)
    \\
    &< 0,
\end{align*}
meaning $\mu_\av < \mu_{\av\circ\left(\pi_k, \pi_{k+1}\right)}$, which corresponds to Property (2) of Assumption 1.

Similarly, if Property \eqref{eq:kappabad} is satisfied, then
Property (2) of Assumption 1 is fulfilled.

If Property \eqref{eq:thetabadoutside} is satisfied,
\begin{align*}
    \mu_\av - \mu_{\av[\pi_{K} := i]}
    &=  \theta_{a_{\pi_K}}\kappa_{\pi_K} - \theta_{i}\kappa_{\pi_K}
    \\
    &= \left(\theta_{a_{\pi_K}} - \theta_{i}\right)\kappa_{\pi_K}
    \\
    &< 0.
\end{align*}
Hence $\mu_\av < \mu_{\av[\pi_{K} := i]}$, which corresponds to Property (3) of Assumption 1.

Finally, if Property \eqref{eq:everythingok} is satisfied, $\mu_\av = \mu^*$.

Overall, either $\av$ is one of the best arms, or $\av$ fulfills Property (2) of Assumption 1, or $\av$ fulfills Property (3) of Assumption 1, which concludes the proof.

\end{proof}

\section{Preliminary to the Analysis of \ouralgo{}}\label{app:prelim}

The analysis of \ouralgo{} requires a control of the number of high deviations, as expressed by Lemma $B.1$ of \cite{Combes2014}. Let us recall this lemma, which we denote Lemma \ref{lem:B1} in current paper. 

\begin{lemma}[Lemma B.1 of \cite{Combes2014}]\label{lem:B1}
Let $i\in [L]$, $k\in[K]$, $\epsilon>0$.
Define $\Fc(T)$ the $\sigma$-algebra generated by $\left(\cv(t)\right)_{t\in [T]}$.
Let $\Lambda\subseteq\NN$ be a random set of instants. Assume that there exists a sequence of random sets $\left(\Lambda(s)\right)_{s\geq1}$ such that (i)  $\Lambda\subseteq\bigcup_{s\geq1}\Lambda(s)$, (ii) for all $s\geqslant 1$ and all $t\in \Lambda(s)$, $T_{i,k}(t)\geq\epsilon s$, (iii) $|\Lambda(s)|\leqslant 1$, and (iv) the event $t\in \Lambda(s)$ is $\Fc_t$-measurable. Then for all $\delta>0$,

$$\EE\left[\sum_{t\geq1} \ind\{t \in \Lambda,  |\hat\rho_{i, k}(t) - \rho_{i, k}| \geqslant \delta \}\right]\\
 \leqslant \frac{1}{\epsilon\delta^2}$$
\end{lemma}

\section{Proof of Theorem \ref{theo:good_leader} (Upper-bound on the Regret of  KL-CombUCB)}\label{app:good_leader}

\begin{proof}[Proof of Theorem \ref{theo:good_leader}]
Let $\av\in \Ac$ be a sub-optimal arm. 
Let $\av^*\in \Ac$ be an optimal arm such that $|\av\setminus\av^*| = K_\av$.

We denote $\bar{K}_\av\defeq |\av^*\setminus\av|$,
$T_\av(t) \defeq \sum_{s = 1}^{t-1} \ind\{\av(s) = \av\}$
the number of time the arm $\av$ has been drawn,
and $T_e(t) \defeq \sum_{s = 1}^{t-1} \ind\{e \in \av(s)\}$ the number of time the element $e$ was in the drawn arm. 

Let decompose the expected number of iterations at which the permutation $\av$ is recommended:
\begin{align*}
\EE\left[\sum_{t=1}^T \ind\{\av(t) = \av\}\right]
    &\leqslant \sum_{e \in \av\setminus\av^*}\EE\left[\sum_{t=1}^T \ind\left\{\av(t) = \av, |\hat\rho_e(t) - \rho_e|\geqslant \frac{\Delta_\av}{2K_\av}  \right\}\right]
\\
    &\quad + \sum_{e \in \av^*\setminus\av}\EE\left[\sum_{t=1}^T \ind\{b_e(t) \leqslant \rho_e \}\right]
    \\
    &\quad +  \EE\left[\sum_{t=|E|}^{T} \ind\left\{\av(t) = \av, \forall e \in \av\setminus\av^*, |\hat\rho_e(t) - \rho_e|< \frac{\Delta_\av}{2K_\av},  \forall e \in \av^*\setminus\av, b_e(t) > \rho_e \right\}\right]
    \\
    &\quad + |E|
    .
\end{align*}
The proof consists in upper-bounding each term on the right-hand side.

\paragraph{First Term}
Let $e \in \av\setminus\av^*$, and denote $A_e = \left\{t\in [T]: \av(t) = \av, |\hat\rho_e(t) - \rho_e|\geqslant \frac{\Delta_\av}{2K_\av}\right\}$.

$A_e \subseteq \bigcup_{s\in \NN} \Lambda_k(s)$, where $\Lambda_k(s) \defeq \{t\in A_e : T_{\av}(t)=s\}$. For any integer value $s$, $|\Lambda_k(s)| \leqslant 1$ as  $T_\av(t)$ increases for each $t\in A_e$. Note that for each $s\in \NN$ and $n\in \Lambda_k(s)$, $T_e(n) \geqslant T_\av(n)=s$. Then, by Lemma \ref{lem:B1}

\begin{align*}
    \EE\left[|A_e|\right]
    &\leq\EE\left[\sum_{t=1}^T \ind\{t \in A_e\}\right]\\
    & = \EE\left[\sum_{t=1}^T \ind\left\{t \in A_e,  |\hat\rho_e(t) - \rho_e| \geqslant \frac{\Delta_\av}{2K_\av} \right\}\right]\\
    & \leqslant \frac{4K_\av^2}{\Delta_\av^2}.
\end{align*}
Hence, $ \sum_{e \in \av\setminus\av^*}\EE\left[\sum_{t=1}^T \ind\left\{\av(t) = \av, |\hat\rho_e(t) - \rho_e|\geqslant \frac{\Delta_\av}{2K_\av}  \right\}\right]
= \sum_{e \in \av\setminus\av^*} \EE\left[|A_e|\right]
\leqslant \frac{4K_\av^3}{\Delta_\av^2}$.

\paragraph{Second Term}
Let $e \in \av^*\setminus\av$, and denote $B_e \defeq \{t\in [T]: b_e(t) \leqslant \rho_e\}$.

By Theorem 10 of \cite{Garivier2011}, $\EE\left[|B_e|\right] = O(\log\log T)$, so $ \sum_{e \in \av^*\setminus\av}\EE\left[\sum_{t=1}^T \ind\{b_e(t) \leqslant \rho_e \}\right] = \OO(\bar{K}_\av\log \log T)$.

\paragraph{Third Term}
Let note $C \defeq \left\{t\in [T]\setminus[|E|]: \av(t) = \av, \forall e \in \av\setminus\av^*, |\hat\rho_e(t) - \rho_e|< \frac{\Delta_\av}{2K_\av},  \forall e \in \av^*\setminus\av, b_e(t) > \rho_e\right\}$.

Let $t\in C$.

At each step of the initialization phase, the algorithm removes at least one element $e$ of the set $\tilde{E}$ of unseen elements. Therefore, the initialization lasts at most $|E|$ iterations. Hence, at iteration $t$, $\av(t)=\av$ is chosen as $\sum_{e\in\av} b_e(t) = \max_{\av'\in\Ac}\sum_{e\in\av'} b_e(t)$.

Then, by Pinsker's inequality and the fact that $t\leqslant T$, and $T_e(t) \geqslant T_\av(t)$ for any $e$ in $\av$,
\begin{align*}
    0
    & \leqslant \sum_{e\in\av} b_e(t) - \sum_{e\in\av^*}  b_e(t)
    \\
    &= \sum_{e\in\av\setminus\av^*} b_e(t) - \sum_{e\in\av^*\setminus\av}  b_e(t)
    \\
    &\leqslant \sum_{e\in\av\setminus\av^*} \hat\rho_e(t) +  \sqrt{\frac{\log(t)+3\log(\log(t))}{2T_e(t)}}
    - \sum_{e\in\av^*\setminus\av} b_e(t)
    \\
    &< \sum_{e\in\av\setminus\av^*} \rho_e + \frac{\Delta_\av}{2K_\av} + \sqrt{\frac{\log(T)+3\log(\log(T))}{2 T_\av(t)}}
    - \sum_{e\in\av^*\setminus\av} \rho_e
    \\
    &\leqslant \sum_{e\in\av} \rho_e - \sum_{e\in\av^*} \rho_e 
    + K_\av \frac{\Delta_\av}{2K_\av}
    + K_\av\sqrt{\frac{\log(T)+3\log(\log(T))}{2 T_\av(t)}} 
    \\
    &= -\Delta_\av  + \frac{2\Delta_\av}{2} +  K_\av\sqrt{\frac{\log(T)+3\log(\log(T))}{2 T_\av(t)}}.
    \\
    &= - \frac{\Delta_\av}{2} +  K_\av\sqrt{\frac{\log(T)+3\log(\log(T))}{2 T_\av(t)}}.
\end{align*}

Hence, $T_\av(t) <  K_\av^2\frac{2\log(T)+6\log(\log(T))}{\Delta_\av^2}$.
Therefore, $C\subseteq \left\{t\in [T]\setminus[|E|]: \av(t) = \av, T_\av(t) < K_\av^2\frac{2\log(T)+6\log(\log(T))}{\Delta_\av^2}\right\}$, and

\begin{align*}
    \EE&\left[\sum_{t=|E|}^{T} \ind\left\{\av(t) = \av, \forall e \in \av\setminus\av^*, |\hat\rho_e(t) - \rho_e|< \frac{\Delta_\av}{2K_\av},  \forall e \in \av^*\setminus\av, b_e(t) > \rho_e \right\}\right]
    \\
    &= \EE\left[|C|\right]
    \\
    &\leqslant \EE\left[\left|\left\{t\in [T]\setminus[|E|]: \av(t) = \av, T_\av(t) < K_\av^2\frac{2\log(T)+6\log(\log(T))}{\Delta_\av^2}\right\}\right|\right]
    \\
    &\leqslant K_\av^2\frac{2\log(T)+6\log(\log(T))}{\Delta_\av^2}.
\end{align*}

\paragraph{Regret upper-bound}
Overall,
\begin{align*}
\EE\left[\sum_{t=1}^T \ind\{\av(t) = \av\}\right]
&\leqslant \frac{4K_\av^3}{\Delta_\av^2}
+ \OO(\bar{K}_\av\log \log T)
+ K_\av^2\frac{2\log(T)+6\log(\log(T))}{\Delta_\av^2}
+ |E|
\\
& = \frac{2K_\av^2}{\Delta_\av^2}\log(T)
+ \OO\left(\left(\bar{K}_\av+\frac{K_\av^2}{\Delta_\av^2}\right)\log \log T\right)
\end{align*}
and
\begin{align*}
R(T)
&=\sum_{\av \in \Ac : \mu_\av \neq \mu^*} \Delta_\av \EE\left[\sum_{t=1}^T \ind\{\av(t) = \av\}\right]
\\
&\leqslant \sum_{\av \in \Ac : \mu_\av \neq \mu^*} \frac{2K_\av^2}{\Delta_\av}\log(T)
+ \OO\left(\left(\bar{K}_\av\Delta_\av+\frac{K_\av^2}{\Delta_\av}\right)\log \log T\right)
\\
&=\OO\left(\frac{|\Ac|K_{max}^2}{\Delta_{\text{min}}}\log T\right),
\end{align*}
which concludes the proof.

\end{proof}

\section{Proof of Lemma \ref{lem:bad_leader} (Upper-bound on the Number of Iterations of \ouralgo{} for which $\tilde\av(t)=\tilde\av\neq\av^*$)}\label{app:bad_leader}

\begin{proof}[Proof of Lemma \ref{lem:bad_leader}]
Let $\tilde\av \in\perm_K^L\setminus\{\av^*\}$ and prove that $\EE\left[\sum_{t=1}^T\ind\{\tilde\av(t)=\tilde\av\}\right]
= \OO\left(\log\log T\right)$.
%As for any ranking of positions $\tilde\piv \in \Pi_\rhov\left(\tilde\av\right)$, $\EE\left[\sum_{t=1}^T\ind\{\tilde\av(t)=\tilde\av, \tilde\piv(t)=\tilde\piv\}\right]\leqslant\EE\left[\sum_{t=1}^T\ind\{\tilde\av(t)=\tilde\av\}\right]$, it will prove Lemma \ref{lem:bad_leader}.

The proof requires notations related to the neighborhood of $\tilde\av$. Let $\Nc \defeq \bigcup_{\piv\in\perm_K^K}\Nc_\piv(\tilde\av)$
be the set of all the potential neighbors of $\tilde\av$. By definition of the neighborhoods,
$$\Nc=\left\{\tilde\av \circ (k,k'):  k,k' \in [K]^2, k>k'\right\} \cup
\left\{\tilde\av[k := i]: k \in [K], i \in [L]\setminus\tilde\av([K])\right\},$$
and its size is $N=K(2L-K-1)/2$.
As $\tilde\av$ is sub-optimal, and due to Assumption 1, for any appropriate ranking of positions $\piv \in \Pi_\rhov\left(\tilde\av\right)$, there exists a recommendation $\av^+$ with a strictly better expected reward than $\tilde\av$ in the neighborhood $\Nc_\piv(\tilde\av)$. We denote
$$\Nc^+\defeq\bigcup_{\piv \in \Pi_\rhov\left(\tilde\av\right)} \left\{\av^+\in\Nc_\piv(\tilde\av) : \mu_{\av^+} = \max_{\av\in\Nc_\piv(\tilde\av)}\mu_\av\right\}$$
the set of such recommendations. We also chose $\epsilon<\min\{1/(2N), 1/L\}$ and note
$$\delta \defeq \min_{\piv \in \Pi_\rhov\left(\tilde\av\right)}
\min_{\av \in \Nc_{\piv}(\tilde\av) \cup \{\tilde\av\}\setminus\Nc^+}
\left(\max_{\av'\in\Nc_\piv(\tilde\av)}\mu_{\av'} - \mu_\av\right).$$

To bound $\EE\left[\ind\{\tilde\av(t)=\tilde\av\}\right]$, we use the decomposition
$\{t \in [T]: \tilde\av(t)=\tilde\av\} \subseteq \bigcup_{\av^+\in \Nc^+} A_{\av^+} \cup B$ where for any permutation $\av^+\in\Nc^+$,
$$A_{\av^+} = \{t : \tilde\av(t)=\tilde\av, T_{\av^+}(t) \geqslant \epsilon \tilde{T}_{\tilde\av}(t) \}$$
and
$$B = \{t : \tilde\av(t)=\tilde\av, \forall \av^+ \in \Ac+, T_{\av^+}(t) < \epsilon \tilde{T}_{\tilde\av}(t) \}.$$
Hence, 
$$\EE\left[\ind\{\tilde\av(t)=\tilde\av\}\right]
\leqslant \sum_{\av^+ \in \Ac+} \EE\left[|A_{\av^+}|\right]
+ \EE\left[|B|\right].$$

\paragraph{Bound on $\EE\left[|A_{\av^+}|\right]$}
Let $\av^+$ be a permutation in $\Nc^+$ and denote $\Kc^+$ the set of positions for which  $\av^+$ and $\tilde\av$ disagree: $\Kc^+=\left\{k\in[K] : a^+_k \neq \tilde{a}_k\right\}$.
The permutation $\av^+$ is in the neighborhood of $\tilde\av$, so either ${\av^+} = \tilde\av \circ (k, k')$ or ${\av^+} = \av[k := i]$, with $k$ and $k'$ in $[K]$, and $ i$ in $[L]$. Overall, $|\Kc^+| \leqslant 2$.

By the design of the algorithm and by definition of $\epsilon$, we have that $\forall t \in A_{\av^+}$, $T_{\tilde\av}(t) \geqslant \tilde{T}_{\tilde\av}(t)/L > \epsilon \tilde{T}_{\tilde\av}(t)$.
Moreover, at the considered iterations $\tilde\av$ is the leader, so 
\begin{align*}
A_{\av^+} &
  \subseteq \left\{t: \tilde\av(t)=\tilde\av, \tilde{T}_{\tilde\av}(t)<\frac{1}{\epsilon} \right\}
  \cup\left\{t: \tilde\av(t)=\tilde\av, \min\{T_{\tilde\av}(t), T_{\av^+}(t)\} \geqslant \epsilon \tilde{T}_{\tilde\av}(t)\geqslant 1, \muh{\tilde{a}} \geqslant \muh{a^+} \right\}
\\
  &\subseteq \left\{t: \tilde\av(t)=\tilde\av, \tilde{T}_{\tilde\av}(t)<\frac{1}{\epsilon} \right\}
  \cup \left\{t: \tilde\av(t)=\tilde\av, \min\{T_{\tilde\av}(t), T_{\av^+}(t)\} \geqslant \epsilon \tilde{T}_{\tilde\av}(t),  \sum_{k\in\Kc^+}\hat\rho_{\tilde{a}_k,k}(t)
\geqslant \sum_{k\in\Kc^+}\hat\rho_{a^+_k,k}(t) \right\}
\\
 &\subseteq \left\{t: \tilde\av(t)=\tilde\av, \tilde{T}_{\tilde\av}(t)<\frac{1}{\epsilon} \right\}
  \\&\quad\cup \left\{t: \tilde\av(t)=\tilde\av, \min\{T_{\tilde\av}(t), T_{\av^+}(t)\} \geqslant \epsilon \tilde{T}_{\tilde\av}(t),
\exists k\in \Kc^+,
 |\hat\rho_{\tilde{a}_{k}, k}(t) - \rho_{\tilde{a}_{k}, k}| \geqslant \frac{\delta}{2|\Kc^+|}
 \text{ or } 
 |\hat\rho_{a^+_{k}, k}(t) - \rho_{a^+_{k}, k}| \geqslant \frac{\delta}{2|\Kc^+|}
\right\}
\\
 &\subseteq \left\{t: \tilde\av(t)=\tilde\av, \tilde{T}_{\tilde\av}(t)<\frac{1}{\epsilon} \right\}
  \cup \bigcup_{k\in\Kc^+}\bigcup_{i\in\left\{\tilde{a}_k, a^+_k\right\}}
 \Lambda_{i, k},
\end{align*}
with $\Lambda_{i, k} \defeq \left\{t: \tilde\av(t)=\tilde\av, \min\{T_{\tilde\av}(t), T_{\av^+}(t)\} \geqslant \epsilon \tilde{T}_{\tilde\av}(t),
 |\hat\rho_{i, k}(t) - \rho_{i, k}| \geqslant \frac{\delta}{2|\Kc^+|}
\right\}$.

Fix $k$ in $\Kc^+$ and $i$ in $\left\{\tilde{a}_k, a^+_k\right\}$.
$\Lambda_{i,k} \subseteq \bigcup_{s\in\NN}\Lambda_{i,k}(s)$, with $\Lambda_{i,k}(s) \defeq \{t\in \Lambda_{i,k}: \tilde{T}_{\tilde\av}(t) = s\}$. $|\Lambda_{i,k}(s)| \leqslant 1$ as $\tilde{T}_{\tilde\av}(t)$ increases for each $t\in \Lambda_{i,k}$.  Note that for each $s\in \NN$ and $n \in \Lambda_{i,k}(s)$, $T_{i,k}(n) \geqslant \min\left\{T_\av(n), T_{\av^+}(n)\right\} \geqslant \epsilon\tilde{T}_{\tilde\av}(n)=\epsilon s$. Then, by Lemma \ref{lem:B1}
\begin{align*}
\EE\left[|\Lambda_{i,k}|\right]
&=\EE\left[\sum_{t=1}^T \ind\{t \in \Lambda_{i,k}\}\right]\\
& = \EE\left[\sum_{t=1}^T \ind\left\{t \in \Lambda_{i,k}, |\hat\rho_{i,k}(t) - \rho_{i,k}| > \frac{\delta}{2|\Kc^+|} \right\}\right]\\
& \leqslant \frac{4|\Kc^+|^2}{\epsilon\delta^2}
\end{align*}
Hence, $\EE\left[|A_{\av^+}|\right] \leqslant \frac{1}{\epsilon} + \sum_{k\in\Kc^+}\sum_{i\in\left\{\tilde{a}_k, a^+_k\right\}} \EE\left[|\Lambda_{i, k}|\right]  \leqslant \frac{1}{\epsilon} + \frac{8|\Kc^+|^3}{\epsilon\delta^2}$.

\paragraph{Bound on $\EE\left[|B|\right]$}
We first split $B$ in two parts: $B=B^{t_0} \cup B_{t_0}^T$, where $B^{t_0}\defeq \{t\in B: \tilde{T}_{\tilde\av}(t)\leqslant t_0\}$, $B_{t_0}^T\defeq \{t\in B: \tilde{T}_{\tilde\av}(t) > t_0\}$, and $t_0$ is chosen as small as possible to satisfy three constraints required in the rest of the proof.

Namely, $t_0 = \max \left\{
\frac{1}{\epsilon},
(1+N)(1-\frac{1}{L}-\epsilon N)^{-1},
\inf \left\{t: 2\sqrt{\frac{\log (t+1) + 3\log(\log (t+1))}{2\epsilon t}} < \frac{\delta}{8}\right\} \right\}$. Note that $t_0$ only depends on $K$, $L$  and $\delta$, and that $(1-\frac{1}{L}-\epsilon N) > 0$ (assuming $L \geqslant 2$) as $\epsilon < 1/(2N)$.

We also define
\begin{itemize}
    \item $D \defeq \bigcup_{(\av,k) \in (\Nc\cup\{\tilde\av\}\setminus\Nc^+)\times[K]}D_{\av,k}$, where
    $D_{\av,k} \defeq \left\{t \in [T]:  \tilde\av(t)=\tilde\av, \av(t)=\av
    , |\hat\rho_{a_k, k}(t) - \rho_{a_k, k}| \geqslant \frac{\delta}{8}\right\},$
    \item $E \defeq \bigcup_{(\av^+,k)\in \Nc^+\times [K]}E_{\av^+,k}$, where
    $E_{\av^+,k} \defeq \{t \in [T]:  \tilde\av(t)=\tilde\av, b_{a^+_{k},k}(t) \leqslant \rho_{a^+_{k},k} \},$
    \item and $F \defeq\{t \in [T]: \tilde\av(t)=\tilde\av, \tilde\piv(t)\notin\Pi_\rhov\left(\tilde\av\right)\}.$
\end{itemize}

Let $t \in B_{t_0}^T$. By construction, \ouralgo{} forces itself to select $\left\lceil \frac{\tilde{T}_{\tilde\av}(t)}{L} \right\rceil$ times the leader $\tilde\av$  between iterations 1 and $t-1$. So, 
$$\tilde{T}_{\tilde\av}(t)  = \left\lceil \frac{\tilde{T}_{\tilde\av}(t)}{L} \right\rceil + \sum_{\av \in \Nc\cup\{\tilde\av\}}T_{\av}^{\tilde\av}(t)$$
where $T_{\av}^{\tilde\av}(t) = \sum_{s=1}^{t-1} \ind\left\{\tilde\av(s)=\tilde\av, \av(s) = \av, \tilde{T}_{\tilde\av}(s)/L \notin \NN\right\}$ is the number of times arm $\av \in \Nc\cup\{\tilde\av\}$ has been played \textbf{normally} (i.e not forced) while $\tilde\av$ was leader, up to time $t-1$. Let prove by contradiction that there is at least one recommendation $\av$ that has been selected \textbf{normally} more than $\epsilon \tilde{T}_{\tilde\av}(t)+1$ times, namely $T_{\av}^{\tilde\av}(t)\geqslant \epsilon \tilde{T}_{\tilde\av}(t)+1$.

Assume that for each recommendation $\av$ in $\Nc\cup\{\tilde\av\}$, $T_{\av}^{\tilde\av}(t) < \epsilon \tilde{T}_{\tilde\av}(t)+1$. Then
\begin{align*}
\tilde{T}_{\tilde\av}(t)
&= \left\lceil \frac{\tilde{T}_{\tilde\av}(t)}{L} \right\rceil + \sum_{\av \in \Nc\cup\{\tilde\av\}}T_{\av}^{\tilde\av}(t)\\
&< 1 + \frac{\tilde{T}_{\tilde\av}(t)}{L}
+ N (\epsilon \tilde{T}_{\tilde\av}(t) +1).
\end{align*}
Therefore
$\tilde{T}_{\tilde\av}(t) (1- \frac{1}{L} - N \epsilon ) < 1 + N$, which contradicts $t\in B_{t_0}^T$.

So, there exists a  recommendation $\av$ such that $T_{\av}^{\tilde\av}(t)\geqslant \epsilon \tilde{T}_{\tilde\av}(t)+1$. Let denote $s'$ the first iteration such that $T_{\av}^{\tilde\av}(s')\geqslant \epsilon \tilde{T}_{\tilde\av}(t)+1$. At this iteration,  $T_{\av}^{\tilde\av}(s') =T_{\av}^{\tilde\av}(s'-1) +1$, meaning that $\tilde\av(s'-1) = \tilde\av$,  $\av(s'-1)=\av$,  $\tilde{T}_{\tilde\av}(s'-1)/L \notin \NN$, and $T_{\av}^{\tilde\av}(s'-1)\geqslant \epsilon \tilde{T}_{\tilde\av}(t)$. Therefore, the set  $\{s \in [t]: \tilde\av(s) = \tilde\av, T_{\av(s)}^{\tilde\av}(s) \geqslant \epsilon \tilde{T}_{\tilde\av}(t),   \tilde{T}_{\tilde\av}(s)/L \notin \NN \}$ is non-empty. We define $\psi(t)$ as the minimum on this set
$$ \psi(t) \defeq \min\left\{s \in [t]: \tilde\av(s) = \tilde\av, T_{\av(s)}^{\tilde\av}(s) \geqslant \epsilon \tilde{T}_{\tilde\av}(t),   \tilde{T}_{\tilde\av}(s)/L \notin \NN \right\}.$$

We note $\av$ the recommendation $\av(\psi(t))$ at iteration $\psi(t)$.
We have $\av \notin \Nc^+$ since for any recommendation $\av^+ \in\Nc^+$, $T_{\av^+}^{\tilde\av}(\psi(t)) \leqslant T_{\av^+}^{\tilde\av}(t) \leqslant T_{\av^+}(t) < \epsilon \tilde{T}_{\tilde\av}(t)$.
Let $\av^+$ be one of the best recommendations in $\Nc_{\tilde\piv\left(\psi(t)\right)}\left(\tilde\av\right)\cup\{\tilde\av\}$, meaning $\mu_{\av^+} = \max_{\av'\in \Nc_{\tilde\piv\left(\psi(t)\right)}\left(\tilde\av\right)\cup\{\tilde\av\}}\mu_{\av'}$,
and let $\Kc$ denote the set of positions for which $\av$ and $\av^+$ disagree. As both recommendations are in  $\Nc_{\tilde\piv\left(\psi(t)\right)}(\tilde\av)\cup\{\tilde\av\}$, $|\Kc|\leqslant 4$.

Let prove by contradiction that $\psi(t) \in D \cup E \cup F$. Assume that $\psi(t) \notin D \cup E \cup F$. 

Since $\psi(t) \notin F$, $\tilde\piv\left(\psi(t)\right)$ belongs to $\Pi_\rhov\left(\tilde\av\right)$ and hence $\av{^+}$ is in $\Nc^+$ and $\sum_k \rho_{a^+_k, k} - \sum_k \rho_{a_k, k} =\mu_{\av^+}-\mu_\av\geqslant \delta$.

Moreover, since $\psi(t) \notin D \cup E$, for each position $k\in[K]$, $ |\hat\rho_{a_k, k}(\psi(t)) - \rho_{a_k, k}| < \frac{\delta}{8}$, and $b_{a^+_{k},k}(\psi(t)) > \rho_{a^+_{k},k} $.

Finally, $T_{\av}(\psi(t)) \geqslant T_{\av}^{\tilde\av}(\psi(t)) \geqslant \epsilon \tilde{T}_{\tilde\av}(t) \geqslant 1$, and therefore $b_{a_k, k}(\psi(t))$ and $\hat\rho_{a_k, k}(\psi(t))$ are properly defined for any position $k\in[K]$.

Then, by Pinsker's inequality and the fact that $\psi(t)\leqslant t$, $\tilde{T}_{\tilde\av}(s)$ is non-decreasing in $s$, and $T_{\av}(\psi(t)) \geqslant \epsilon \tilde{T}_{\tilde\av}(t) $, 
\begin{align*}
\sum_{k} b_{a_k, k}(\psi(t)) - \sum_{k}  b_{a^+_k, k}(\psi(t))
&= \sum_{k\in\Kc} b_{a_k, k}(\psi(t)) - b_{a^+_k, k}(\psi(t))
\\
&\leqslant \sum_{k\in\Kc} \hat\rho_{a_k, k}(\psi(t)) +  \sqrt{\frac{\log(\tilde{T}_{\tilde\av}(\psi(t))+1)+3\log(\log(\tilde{T}_{\tilde\av}(\psi(t))+1))}{2T_{\av}(\psi(t))}} - b_{a^+_k, k}(\psi(t))
\\
&< \sum_{k\in\Kc} \rho_{a_k, k} + \frac{\delta}{8} + \sqrt{\frac{\log(\tilde{T}_{\tilde\av}(t)+1)+3\log(\log(\tilde{T}_{\tilde\av}(t)+1))}{2\epsilon \tilde{T}_{\tilde\av}(t)}} - \rho_{a^+_k, k}
\\
&\leqslant \sum_{k\in\Kc} \rho_{a_k, k} + \frac{\delta}{8} + \frac{\delta}{8} - \rho_{a^+_k, k}
\\
&\leqslant \sum_k \rho_{a_k, k} - \sum_k \rho_{a^+_k, k}  + |\Kc| \cdot2\frac{\delta}{8}
\\
&\leqslant -\delta  + 8\frac{\delta}{8}
\\
&=0,
\end{align*}
which contradicts the fact that $\av$ is played at iteration $\psi(t)$. So $\psi(t) \in D \cup E \cup F$.

Overall, for any $t\in B_{t_0}^T$,  $\psi(t) \in D \cup E \cup F$. So, $ B_{t_0}^T \subseteq  \bigcup_{n\in D \cup E \cup F} B_{t_0}^T\cap\left\{t\in [T]: \psi(t)=n \right\}$. Let $n$ be in $D \cup E \cup F$. For any $t$ in $B_{t_0}^T\cap\left\{t\in [T]: \psi(t)=n \right\}$, $T_{\av(n)}^{\tilde\av}(n) = \lceil\epsilon \tilde{T}_{\tilde\av}(t)\rceil$ and $\tilde{T}_{\tilde\av}(t+1)=\tilde{T}_{\tilde\av}(t)+1$. So $|B_{t_0}^T\cap\left\{t\in [T]: \psi(t)=n \right\}| < 1/\epsilon+1$.
Overall,
$$\EE\left[|B|\right]
\leqslant t_0 + \EE\left[|B_{t_0}^T|\right]
\leqslant t_0 + \left(1/\epsilon+1\right)(\EE\left[|D|\right]+\EE\left[|E|\right]+\EE\left[|F|\right]).$$

It remains to upper-bound $\EE\left[|D|\right]$, $\EE\left[|E|\right]$, and $\EE\left[|F|\right]$ to conclude the proof.

\paragraph{Bound on $\EE\left[|D|\right]$}
The upper-bound on $\EE\left[|D|\right]$ is obtained with the same strategy as the last step in the proof of the upper-bound on $\EE\left[|A_{\av^+}|\right]$. Let $ \av$ be a recommendation in $\Nc\cup\{\tilde\av\}\setminus\Nc^+$, and $k \in [K]$ be a position. $D_{\av,k} \subseteq \bigcup_{s\in \NN} \Lambda_{\av,k}(s)$, where $\Lambda_{\av,k}(s) \defeq \{t\in D_{\av,k} : T_{\av}(t)=s\}$. $|\Lambda_{\av,k}(s)| \leqslant 1$ as  $T_{\av}(t)$ increases for each $t\in D_{\av,k}$. Note that for each $s\in \NN$ and $n\in \Lambda_{\av,k}(s)$, $T_{a_k, k}(n) \geqslant T_{\av}(n)=s$. Then, by Lemma \ref{lem:B1}

\begin{align*}
    \EE\left[|D_{\av,k}|\right]
    &\leq\EE\left[\sum_{t=1}^T \ind\{t \in D_{\av,k}\}\right]\\
    & = \EE\left[\sum_{t=1}^T \ind\left\{t \in D_{\av,k},  |\hat\rho_{a_k, k}(t) - \rho_{a_k, k}| \geqslant \frac{\delta}{8} \right\}\right]\\
    & \leqslant \frac{64}{\delta^2}
\end{align*}
Hence, $\EE\left[|D|\right] \leq
\sum_{(\av,k) \in (\Nc\cup\{\tilde\av\}\setminus\Nc^+)\times[K]}\EE\left[|D_{\av,k}|\right]
\leqslant \frac{64(N+1)K}{\delta^2}$.

\paragraph{Bound on $\EE\left[|E|\right]$}

By Theorem 10 of \cite{Garivier2011}, $\EE\left[|E_{\av^+,k}|\right] = O(\log(\log(T)))$, so 
$\EE\left[|E|\right]
\leqslant \sum_{(\av^+,k)\in \Nc^+\times [K]}
\EE\left[|E_{\av^+,k}|\right] = O(|\Nc^+|K\log(\log(T)))$.

\paragraph{Bound on $\EE\left[|F|\right]$}

By Lemma \ref{lem:badordering}, $\EE\left[|F|\right] = \EE\left[\sum_{t=1}^T\ind\left\{\tilde\av(t)=\tilde\av,\\ \tilde\piv(t)\notin\Pi_\rhov\left(\tilde\av\right) \right\}\right]
= \OO\left(1\right).$

Overall $\EE\left[\ind\{\tilde\av(t)=\tilde\av\}\right] \leqslant
\frac{|\Kc^+|}{\epsilon}
+ \frac{8|\Kc^+|^3|\Nc^+|}{\epsilon\delta^2}
+ t_0
+ \left(\frac{1}{\epsilon}+1\right)\frac{64(N+1)K}{\delta^2}
+ \OO\left(\frac{|\Nc^+|K}{\epsilon}\log\log T\right)
+\OO(1)
= \OO\left(\frac{|\Nc^+|K}{\epsilon}\log\log T\right)$, which concludes the proof.
\end{proof}

\section{Proof of Lemma \ref{lem:badordering} (Upper-bound on the Number of Iterations of \ouralgo{} for which $\tilde\piv(t) \notin \Pi_\rhov(\tilde\av)$)}\label{app:badordering}

\begin{proof}[Proof of Theorem \ref{lem:badordering}]
Let $\tilde\av$ be a $K$-permutation of $L$ items. If $\Pi_\rhov\left(\tilde\av\right)$ contains all the permutations of $K$ elements, the set $\left\{t:\tilde\av(t)=\tilde\av, \tilde\piv(t)\notin \Pi_\rhov\left(\tilde\av\right)\right\}$ is empty.

Otherwise, let denote $\delta$ the smallest non-zero gap between the probability of click at position $k$ and the probability of click at position $k'\neq k$: $\delta\defeq\min \left\{\rho_{\tilde{a}_k,k}-\rho_{\tilde{a}_{k'},k'} : (k,k')\in[K]^2, \rho_{\tilde{a}_k,k}-\rho_{\tilde{a}_{k'},k'}>0\right\}$. The gap $\delta$ is the minimum on a finite set, so $\delta>0$.

By definition of $\tilde\pi(t)$,
$\hat\rho_{\tilde{a}_{\tilde\pi_1(t)}(t),\tilde\pi_1(t)}(t) \geqslant \hat\rho_{\tilde{a}_{\tilde\pi_2(t)}(t),\tilde\pi_2(t)}(t) \geqslant \dots \geqslant \hat\rho_{\tilde{a}_{\tilde\pi_K(t)}(t),\tilde\pi_K(t)}(t),$
so,
\begin{align*}
    \left\{t:\tilde\av(t)=\tilde\av, \tilde\piv(t)\notin\Pi_\rhov\left(\tilde\av\right)\right\}
    &= \bigcup_{\tilde\piv\in\perm_K^K}\bigcup_{k\in[K-1]}
    \left\{t:\tilde\av(t)=\tilde\av, \tilde\piv(t)=\tilde\piv,
    \rho_{\tilde{a}_{\tilde\pi_k}, \tilde\pi_k} < \rho_{\tilde{a}_{\tilde\pi_{k+1}}, \tilde\pi_{k+1}}\right\}
    \\
    &\subseteq \bigcup_{\tilde\piv\in\perm_K^K}\bigcup_{k\in[K-1]}
    \left\{t:\tilde\av(t)=\tilde\av, \tilde\piv(t)=\tilde\piv, 
    \substack{
    |\hat\rho_{\tilde{a}_{\tilde\pi_k}, \tilde\pi_k}(t)
        - \rho_{\tilde{a}_{\tilde\pi_k}, \tilde\pi_k}| > \frac{\delta}{2}\\
    \text{ or }|\hat\rho_{\tilde{a}_{\tilde\pi_{k+1}}, \tilde\pi_{k+1}}(t)
        - \rho_{\tilde{a}_{\tilde\pi_{k+1}}, \tilde\pi_{k+1}}| > \frac{\delta}{2}
    }
    \right\}
    \\
    &= \bigcup_{\tilde\piv\in\perm_K^K}\bigcup_{k\in[K]} \Lambda_{\tilde\piv,k},
\end{align*}
with
$\Lambda_{\tilde\piv,k} \defeq \left\{t:\tilde\av(t)=\tilde\av, \tilde\piv(t)=\tilde\piv, 
    |\hat\rho_{\tilde{a}_{\tilde\pi_k}, \tilde\pi_k}(t)
        - \rho_{\tilde{a}_{\tilde\pi_k}, \tilde\pi_k}| > \frac{\delta}{2}\right\},$
for any ranking of positions $\tilde\piv\in\perm_K^L$ and any rank $k\in [K]$.

Let $\tilde\piv\in\perm_K^L$ be a ranking of positions, and $k\in[K]$ be a rank.
$\Lambda_{\tilde\piv,k} \subseteq \bigcup_{s\in\NN}\Lambda_{\tilde\piv,k}(s)$, with $\Lambda_{\tilde\piv,k}(s) \defeq \{t\in \Lambda_{\tilde\piv,k}: \tilde{T}_{\tilde\av}(t) = s\}$. $|\Lambda_{\tilde\piv,k}(s)| \leqslant 1$ as $\tilde{T}_{\tilde\av}(t)$ increases for each $t\in \Lambda_{\tilde\piv,k}$.  Note that for each $s\in \NN$ and $n \in \Lambda_{\tilde\piv,k}(s)$, $T_{\tilde{a}_{\tilde\pi_k}, \tilde\pi_k}(n) \geqslant T_{\tilde\av}(n)\geqslant \tilde{T}_{\tilde\av}(n)/L=s/L$. Then, by Lemma \ref{lem:B1}
\begin{align*}
\EE\left[|\Lambda_{\tilde\piv,k}|\right]
&=\EE\left[\sum_{t=1}^T \ind\{t \in \Lambda_{\tilde\piv,k}\}\right]\\
& = \EE\left[\sum_{t=1}^T \ind\left\{t \in \Lambda_{\tilde\piv,k}, |\hat\rho_{\tilde{a}_{\tilde\pi_k}, \tilde\pi_k}(t) - \rho_{\tilde{a}_{\tilde\pi_k}, \tilde\pi_k}| > \frac{\delta}{2} \right\}\right]\\
& \leqslant \frac{4L}{\delta^2}
\end{align*}

Hence,
\begin{align*}
\EE\left[\sum_{t=1}^T\ind\{\tilde\av(t)=\tilde\av, \tilde\piv(t)\notin\Pi_\rhov\left(\tilde\av\right) \}\right]
&\leqslant \sum_{\tilde\piv\in\perm_K^K}\sum_{k\in[K]} \EE\left[\Lambda_{\tilde\piv,k}\right]
\\
&\leqslant \frac{4LKK!}{\delta^2}
\\
&= \OO\left(LKK!\right),
\end{align*}
which concludes the proof.

\end{proof}

\begin{algorithm}[tb]
\caption{KL-ComUCB1 (generic version)}\label{alg:KL-ComUCB1_generic}
\begin{algorithmic}
\REQUIRE set of elements $E$, set of arms $\Ac$
\STATE $t\gets 1$
\WHILE{$\{e\in E:T_e(t)=0\} \neq \varnothing$}
\STATE $\tilde{E} \gets \{e\in E: T_e(t)=0\}$
\STATE $\tilde{\Ac} \gets \{\av\in\Ac :  \av \cap \tilde{E}\neq\varnothing\}$
\STATE recommend $\displaystyle\av(t) = \argmax_{\av \in \tilde\Ac}
\sum_{e\in \av}b_{e}(t)$
\STATE observe the weights $\left[w_e(t) : e\in\av\right]$
\STATE $t\gets t+1$
\ENDWHILE
\STATE $t_0\gets t$
\FOR{$t =  t_0, t_0+1, \dots$}
\STATE recommend $\displaystyle\av(t) = \argmax_{\av \in \Ac}
\sum_{e\in \av}b_{e}(t)$  
\STATE observe the weights $\left[w_e(t) : e\in\av\right]$
\ENDFOR
\end{algorithmic}
\end{algorithm}

\section{KL-CombUCB and its Application to PBM Setting} \label{app:KL-Comb_to_PBM}
In this section we first define the generic combinatorial semi-bandit algorithm KL-CombUCB and we compare two upper-bounds on its regret. Then, we present the application of KL-CombUCB to PBM setting and discuss its relation to \ouralgo{}.

\subsection{KL-CombUCB for Generic Setting}

CombUCB1 \cite{Kveton2015CombUCB} is a bandit algorithm handling the following combinatorial setting. Let $E$ be a set of elements and $\Ac\subseteq\{0,1\}^E$ be a set of arms, where each arm $\av$ is a subset of $E$.
Following the terminology used in \cite{Kveton2015CombUCB}, $E$ is the \emph{ground set} and $\Ac$ the \emph{feasible set}. 
At each iteration, the bandit algorithm chooses a subset of elements $\av\in\Ac$ and receives the reward $\sum_{e \in \av} w_e$, where $\wv$ is an independent draw of a distribution $\nu$ on $[0,1]^E$. Given these assumptions, CombUCB1 chooses an arm $\av(t)$ at each iteration, aiming at minimizing the total regret defined as usual.

%The rest of the exposition requires more notations. 
We denote $\rho_e\defeq\EE_{\wv\sim \nu}\left[w_e\right]$ the expected reward associated to element $e$,
$\mu_\av\defeq \EE_{\wv\sim \nu}\left[\sum_{e \in \av} w_e\right]=\sum_{e\in\av}\rho_e$ the expected reward when choosing the arm $\av\in\Ac$,
and $\mu^*\defeq\max_{\av\in \Ac}\mu_\av$ the best expected reward.
We also denote $\Delta_\av \defeq \mu^*-\mu_\av$ the gap between the best expected reward and the reward of an arm $\av$,
and $\Delta_{min} \defeq \min_{\av \in\Ac:\Delta_\av>0} \Delta_\av$ the smallest gap of a suboptimal arm.
Finally,
$K\defeq\max_{\av\in\Ac}|\av|$ denotes the maximum size of an arm (meaning the maximum number of chosen elements),
$K_\av \defeq \min_{\av^*\in\Ac: \mu_{\av^*}=\mu^*} |\av\setminus\av^*|$ is the smallest number of elements to remove from $\av$ to get an optimal arm,
and $K_{max}\defeq\max_{\av \in\Ac: \mu_\av\neq\mu^*} K_\av$ is its lager value.

In our paper, we use the Kullback-Leibler variation of CombUCB1 which chooses the arm based on the index $b_e(t)$ (defined hereafter) instead of the usual confidence upper-bound derived from the Hoeffding’s inequality. The corresponding algorithm (KL-CombUCB) also assumes that the weight-vector $\wv(t)$ is in $\{0,1\}^E$. KL-CombUCB is depicted by Algorithm \ref{alg:KL-ComUCB1_generic} which uses the following notations. At each iteration $t$,
we denote 
$$\hat\rho_e(t) \defeq \frac{1}{T_e(t)}\sum_{s = 1}^{t-1} \ind\{e \in \av(s)\}w_e(s)$$
the average number of clicks obtained by the element $e$, where
$$T_e(t) \defeq \sum_{s = 1}^{t-1} \ind\{e \in \av(s)\}$$
is the number of times element $e$ has been selected; $\hat\rho_e(t)\defeq0$ when $T_e(t)=0$.
The statistics $\hat\rho_e(t)$ are paired with their respective \emph{indices} $$b_e(t) \defeq f\left(\hat\rho_e(t), T_e(t), t\right),$$
where
$f(\hat\rho, s, t)$ stands for $$\sup \{p\in[\hat\rho,1]: s\times\KL(\hat{\rho}, p) \leq \log (t) + 3 \log(\log (t))\},$$
with
$$\KL(p,q) \defeq p \log \left(\frac{p}{q}\right) + (1-p)\log \left(\frac{1 - p}{1 - q}\right)$$
the \emph{Kullback-Leibler divergence} from a Bernoulli distribution of mean $p$ to a Bernoulli distribution of mean $q$;
$f(\hat\rho, s, t) \defeq 1$ when $\hat{\rho}=1$, $s=0$, or $t=0$. 

\citeauthor{Kveton2015CombUCB} prove that the regret of CombUCB1 is upper-bounded by $\OO\left(|E|K/\Delta_{min}\log T\right)$, and a similar proof would lead to the same upper-bound for KL-CombUCB. In our paper we prove in Theorem \ref{theo:good_leader} a completely different regret upper-bound for KL-CombUCB: $\OO\left(|\Ac|K_{max}^2/\Delta_{min}\log T\right)$. For most combinatorial bandit settings, this new bound is useless since $|\Ac| \gg |E|$, and $K_{max} \approx K$. However, the analysis of \ouralgo{} involves an application of KL-CombUCB to a setting where the new bound is smaller than the standard one as $|\Ac| = |E|-1$ and $K_{max}=2$.

\begin{algorithm}[tb]
\caption{KL-ComUCB1 (applied to PBM)}\label{alg:KL-ComUCB1}
\begin{algorithmic}
\REQUIRE number of items $L$, number of positions $K$
\FOR{$t =  1, 2, \dots, L$}
\STATE recommend $\displaystyle\av(t) = \left(((t -1)\% L) + 1, (t\% L) + 1, \dots, ((t +K-2) \% L) + 1\right)$  
\STATE observe the clicks-vector $\cv(t)$
\ENDFOR
\FOR{$t =  L+1, L+2, \dots$}
\STATE recommend $\displaystyle\av(t) = \argmax_{\av \in \perm_K^L}
\sum_{k=1}^Kb_{a_k, k}(t)$  
\STATE observe the clicks-vector $\cv(t)$
\ENDFOR
\end{algorithmic}
\end{algorithm}

\subsection{KL-CombUCB Applied to PBM Setting}

In the experiments (Section 6), we apply KL-CombUCB to PBM bandit setting by choosing the \emph{ground set} $E = [L]\times[K]$, the \emph{feasible set} $\Theta=\{\{(a_k,k): k \in [K]\}:\av\in\perm_K^L\}$, and the \emph{expected weights} $\rho_{(i,k)}=\theta_i\kappa_k$ for any ``element" $(i,k)\in E$. Note that the observed weights of the generic setting correspond to the clicks-vector in the PBM setting. 

The corresponding algorithm, depicted by Algorithm \ref{alg:KL-ComUCB1}, recommends at each iteration $t$ the best permutation given the indices $b_{i,k}(t)$ defined for \ouralgo{}. This optimization problem
is a \emph{linear sum assignment problem} which is solvable in $\OO\left(K^2(L+\log K)\right)$ time \cite{Ramshaw2012}. Note the close relationship with \ouralgo{}:
\begin{itemize}
    \item both algorithms solve a linear sum assignment problem, they only differ from the metric to optimize: $\sum_{k=1}^K\hat\rho_{a_k, k}(t)$ for \ouralgo{} vs. $\sum_{k=1}^Kb_{a_k, k}(t)$ for KL-CombUCB;
    \item both algorithms recommend the best permutation $\av$ regarding  $\sum_{k=1}^Kb_{a_k, k}(t)$, they only differ from the considered set of permutations:  $\{\tilde\av(t)\}\cup\Nc_{\tilde\piv(t)}\left(\tilde\av(t)\right)$ for \ouralgo{} vs. $\perm_K^L$ for KL-CombUCB.
\end{itemize}
 
By considering a larger set of permutations, KL-ComUCB1 suffers a $\OO(LK^2/\Delta_{min}\log T)$ regret (by applying \cite{Kveton2015CombUCB} bound), which is higher than the upper-bound on the regret of \ouralgo{} by a factor $K^2$.

\section{\ouralgofull{}: OSUB on a Static Graph}\label{app:fgrab}

\begin{algorithm}[tb]
\caption{\ouralgofull{}: \ouralgofulllong{}}\label{alg:S-GRAB}
\begin{algorithmic}
\REQUIRE number of items $L$, number of positions $K$
\STATE $\gamma\gets K(2L-K-1)/2$
\FOR{$t =  1, 2, \dots$}
\STATE $\displaystyle\tilde\av(t) \gets \argmax_{\av \in \perm_K^L}
\sum_{k=1}^K \hat\rho_{a_k,k}(t)$
\STATE
$\displaystyle
\text{recommend }
\av(t) =\begin{cases}
 \tilde\av(t)
 & \text{, if } \frac{\Tilde{T}_{\tilde\av(t)}(t)}{\gamma+1} \in \mathds{N}, \\
 \displaystyle \argmax_{\av \in \{\tilde\av(t)\}\cup\Nc_G(\tilde\av(t))}
 \sum_{k=1}^K b_{a_k, k}(t)
% -
 %\sum_{k=1}^K
% b_{\tilde{a}_k(t), k}
& \text{, otherwise}
\end{cases} $
\\
where $\Nc_G(\av) = \left\{\av \circ (k,k'):  k,k' \in [K]^2, k>k'\right\} \cup
\left\{\av[k := i]: k \in [K], i \in [L]\setminus\av([K])\right\}$
\STATE observe the clicks vector $\cv(t)$
\ENDFOR
\end{algorithmic}
\end{algorithm}

The algorithm \ouralgofull{}, depicted in Algorithm \ref{alg:S-GRAB}, is similar to \ouralgo{} except that it explores a static graph $G=(E, V)$ defined by
\begin{align*}
V&\defeq\perm_K^L,\\
E &\defeq
\left\{(\av, \av \circ (k,k')):  k,k' \in [K]^2, k>k'\right\}
\cup\left\{(\av, \av[k:= i]):  k\in [K], i \in [L]\setminus\av([K])\right\}.
\end{align*}

This graph is chosen to ensure that with PBM setting any sub-optimal recommendation has a strictly better recommendation in its neighborhood given $G$. This graph is fixed and does not require the knowledge of a mapping $\cal P$, but its degree is also about $K$ times larger than the degree of the graphs handled by \ouralgo{}. 

As for \ouralgo{}, any recommendation in the neighborhood of the leader given $G$ differs with the leader at, at most two positions. Therefore a proof similar to the one of Theorem \ref{theo:osrubpbm} ensures that \ouralgofull{}'s regret is upper-bounded by $\OO\left(LK/\Delta_{min}\log T\right)$. This regret upper-bound is higher than \ouralgo{}'s one by a factor $K$ due to the larger size of the considered neighborhoods. However, this regret remains smaller than KL-CombUCB's one by a factor $K$ thanks to the bounded number of differences between the leader and the arm played.

%\bibliography{bib.bib}
%\bibliographystyle{icml2021}
